# Supplementary material for: Gaussian Fluids: A Grid-Free Fluid Solver based on Gaussian Spatial Representation
Source: arXiv:2405.18133 source file (2025-07-09)
Supplement: Supplementary file 1 [file _appendix.tex]

%%
%% If your work has an appendix, this is the place to put it.
\appendix

% \begin{comment}
\twocolumn[
% \begin{center}
{\Huge \sffamily Gaussian Fluids: A Grid-Free Fluid Solver based on Gaussian Spatial Representation} \vspace{12pt}\newline
{\Huge \sffamily Supplementary	}\newline
        \vspace{12pt}
		% {\LARGE \newline SUBMISSION ID: 290}
		% \subsection*{\newline 
		% {\LARGE aaa bbb,} ccc  \newline
        % {\LARGE aaa bbb,} ccc  \newline
        % {\LARGE aaa bbb,} ccc  \newline
		% }
		%\vspace{-8pt}
% \end{center}
  \vspace{12pt}
]
%\appendix
%\section*{Appendix}
%\label{app:detail}
% \end{comment}

\noindent
% \section{Efficient Implementation of GSR}

% We apply a hash grid to accelerate the neighbor search similar to SPH solvers. Since $G_i(\boldsymbol x)\ge c$ is equivalent to $(\boldsymbol x-\mu_i)^\top\boldsymbol\Sigma_i^{-1}(\boldsymbol x-\mu_i)\le-2\ln c$, and we have
% \begin{align}
%     (\boldsymbol x-\mu_i)^\top\boldsymbol R_i\boldsymbol S_i^{-1}\boldsymbol S_i^{-1}\boldsymbol R_i(\boldsymbol x-\mu_i)\ge\min(\boldsymbol s_i^{-1})^2\|\boldsymbol x-\mu_i\|^2,
% \end{align}
% hence for all $\boldsymbol x$ such that $G_i(\boldsymbol x)\ge c$, $\min(\boldsymbol s_i^{-1})^2\|\boldsymbol x-\mu_i\|^2\le-2\ln c$, i.e. $\|\boldsymbol x-\mu_i\|\le\sqrt{-2\ln c}\max(\boldsymbol s_i)$. Thus it is safe to set the grid cell size to $\sqrt{-2\ln c}\max(\boldsymbol s_1,\cdots,\boldsymbol s_n)$. When querying the value or gradient of the GSR on $\boldsymbol x$, we check all the particles in the cell in which $\boldsymbol x$ is and its neighboring cells.

% Note that the grid cell size may change as the particles deform. We set a lower bound of the grid cell size to prevent the algorithm from accessing a grid that has not been allocated from the memory. We need to reinitialize the grid data each time we update the parameters of the GSR.
\section{Parameter Initialization for GSR}

We adopt an adaptive approach to set the initial values of the parameters of GSR. We first divide the domain by a grid with cell length $a$ and place the Gaussian kernels at its nodes. The cell length $a$ is chosen such that the particle number falls in a legitimate range.
Next, we determine the particle size by setting
\begin{equation}
    \boldsymbol s_i=\frac a{\sqrt{-2\ln c}}\boldsymbol 1
\end{equation}
so that the non-zero domain of each kernel is a ball with radius $h=\sqrt{-2\ln c}\cdot s=a$, where $\boldsymbol 1\in\mathbb R^d$ is a vector with all elements one.
We then set other parameters to the most trivial value, i.e. $\boldsymbol v_i=\boldsymbol 0$, $\theta_i=0$ for 2D and $\boldsymbol r_i=\begin{bmatrix}1&0&0&0\end{bmatrix}^\top$ for 3D.

\section{Settings of all Examples}

The normal of the domain boundary points inward.

% \xing{
\subsection{Taylor-Green Vortex}
\begin{itemize}
    \item Domain: $\mathcal D=[0,2\pi]\times[0,2\pi]$.
    \item Initial velocity field:
    \begin{equation}
        \boldsymbol u(\boldsymbol x)=\begin{bmatrix}\sin x\cos y\\-\cos x\sin y\end{bmatrix}.
    \end{equation}
    \item Boundary condition: Second type condition on $\partial\mathcal D$ with $f=0$.
\end{itemize}
% }

\subsection{Taylor Vortex}
\begin{itemize}
    \item Domain: $\mathcal D=[-5,5]\times[-5,5]$.
    \item Initial velocity field:
    \begin{align}
        \boldsymbol u(\boldsymbol x)=&\frac Ua\exp\left\{\frac 12\left(1-\frac{\|\boldsymbol x-\boldsymbol x_1\|^2}{a^2}\right)\right\}\begin{bmatrix}y_1-y\\x-x_1\end{bmatrix}+\notag\\
        &\frac Ua\exp\left\{\frac 12\left(1-\frac{\|\boldsymbol x-\boldsymbol x_2\|^2}{a^2}\right)\right\}\begin{bmatrix}y_2-y\\x-x_2\end{bmatrix},
    \end{align}
    where $U=3$, $a=0.5$, $\boldsymbol x_1=(x_1,y_1)^\top=(-0.8,0)^\top$, $\boldsymbol x_2=(x_2,y_2)^\top=(0.8,0)^\top$.
    \item Boundary condition: Second type condition on $\partial\mathcal D$ with $f=0$.
\end{itemize}

\subsection{Leapfrog 2D}

We define the velocity of a 2D vortex placed at $\boldsymbol z=(z_x,z_y)^\top$ with strength $U$ and radius $a$ as
\begin{align}
    \boldsymbol u_\mathrm{vort}(\boldsymbol x;\boldsymbol z,U,a)=\frac U{(r+\varepsilon)^2}\left(1-\mathrm e^{-\left(\frac{r+\varepsilon}a\right)^2}\right)\begin{bmatrix}z_y-y\\x-z_x\end{bmatrix},
\end{align}
where $r=\|\boldsymbol x-\boldsymbol z\|$, $\varepsilon=10^{-6}$.

\begin{itemize}
    \item Domain: $\mathcal D=[-5,5]\times[-5,5]$.
    \item Initial velocity field:
    \begin{align}
        \boldsymbol u(\boldsymbol x)=&\boldsymbol u_\mathrm{vort}(\boldsymbol x;\boldsymbol x_1,U_0,a_0)+\boldsymbol u_\mathrm{vort}(\boldsymbol x;\boldsymbol x_2,U_0,a_0)+\\\notag
        &\boldsymbol u_\mathrm{vort}(\boldsymbol x;\boldsymbol x_3,-U_0,a_0)+\boldsymbol u_\mathrm{vort}(\boldsymbol x;\boldsymbol x_4,-U_0,a_0),
    \end{align}
    where $\boldsymbol x_1=(-3,-3)^\top$, $\boldsymbol x_2=(-1,-3)^\top$, $\boldsymbol x_3=(1,-3)^\top$, $\boldsymbol x_4=(3,-3)^\top$, $U_0=0.5$, $a_0=0.3$.
    \item Boundary condition: Second type condition on $\partial\mathcal D$ with $f=0$.
\end{itemize}

\subsection{Vortices Pass}

% \begin{itemize}
%     \item Domain: $\mathcal D=[0,1]\times[0,1]$.
%     \item Initial velocity field:
%     \begin{equation}
%         \boldsymbol u(\boldsymbol x)=\boldsymbol u_\mathrm{vort}(\boldsymbol x;\boldsymbol x_1,U_0,a_0)+\boldsymbol u_\mathrm{vort}(\boldsymbol x;\boldsymbol x_2,-U_0,a_0),
%     \end{equation}
%     where $\boldsymbol x_1=(0.1,0.525)^\top$, $\boldsymbol x_2=(0.1,0.475)^\top$, $U_0=0.005$, $a_0=0.03$.
%     \item Boundary condition: Second type condition on $\partial\mathcal D\cup\partial\mathcal B_1\cup\partial\mathcal B_2$ with $f=0$, where $\mathcal B_1$ is a 2D ball with center $(0.5,0.27)$ and radius $\frac{60}{511}$, $\mathcal B_2$ is a 2D ball with center $(0.5,0.73)$ and radius $\frac{60}{511}$.
% \end{itemize}
\xing{
We define the velocity induced by a vortex particle at $\boldsymbol z=(z_x,z_y)^\top$ with strength $U$ as
\begin{equation}
    \boldsymbol u_\mathrm p(\boldsymbol x;\boldsymbol z,U)=\frac U{r^2+\varepsilon_\mathrm p}\begin{bmatrix}y-z_y\\z_x-x\end{bmatrix},
\end{equation}
where $r=\|\boldsymbol x-\boldsymbol z\|$, $\varepsilon_\mathrm p=0.1$.
}
\xing{
\begin{itemize}
    \item Domain: $\mathcal D=[-5,5]\times[-5,5]$.
    \item Initial velocity field: We place some vortex particles near to the two vortices' centers. Denote their positions as $\boldsymbol z_1,\cdots,\boldsymbol z_m$, their strengths $U_1,\cdots,U_m$, the initial velocity field is
    \begin{equation}
        \boldsymbol u(\boldsymbol x)=\sum_{i=1}^m\boldsymbol u_\mathrm p(\boldsymbol x;\boldsymbol z_i,U_i).
    \end{equation}
    Note that all the vortex particles have strengths with a same absolute value $0.0416666679084301$.
    \item Boundary condition: Second type condition on $\partial\mathcal D\cup\partial\mathcal B_1\cup\partial\mathcal B_2$ with $f=0$, where $\mathcal B_1$ is a 2D ball with center $(0,1)$ and radius $0.25$, $\mathcal B_2$ is a 2D ball with center $(0,-1)$ and radius $0.25$.
\end{itemize}
}

\subsection{Karman Vortex Street}
\label{supp:sec:karman}

\begin{itemize}
    \item Domain: $\mathcal D=[-1.10321, 1.906778]\times[-0.598466, 0.60349]$.
    \item Initial velocity field: $\boldsymbol u(\boldsymbol x)=\begin{bmatrix}0.5&0\end{bmatrix}^\top$.
    \item Boundary condition: The boundary condition can be divided into four parts.

    First type condition on $\partial\mathcal B$ with $\boldsymbol u_\mathrm b=\boldsymbol 0$, where $\partial\mathcal B$ is a 2D ball with center $(-0.80356845, -0.00502235)$ and radius $0.04553178393357534$.

    Second type condition at the top and bottom boundary of the domain with $f=0$.

    Second type condition at the left boundary of the domain with $f=0.5$ (inflow condition).

    Second type condition at the right boundary of the domain with $f=-0.5$ (outflow condition).
\end{itemize}

\subsection{Leapfrog 3D}

We denote the velocity of a vortex ring with center at $\boldsymbol z$, facing direction $\boldsymbol n$, radius $r$, thickness $a$ and strength $U$ as $\boldsymbol u_\mathrm{ring}(\boldsymbol x;\boldsymbol z,\boldsymbol n,r,a,U)$.

\begin{itemize}
    \item Domain: $\mathcal D=[0,1]\times[0,1]\times[0,1]$.
    \item Initial velocity field:
    \begin{equation}
        \boldsymbol u(\boldsymbol x)=\boldsymbol u_\mathrm{ring}(\boldsymbol x;\boldsymbol x_1,\boldsymbol n_0,r_1,a_0,U_0)+\boldsymbol u_\mathrm{ring}(\boldsymbol x;\boldsymbol x_2,\boldsymbol n_0,r_2,a_0,U_0),
    \end{equation}
    where $\boldsymbol x_1=(0.75,0.5,0.5)^\top$, $r_1=\frac 16$, $\boldsymbol x_2=(0.85,0.5,0.5)^\top$, $r_2=\frac 7{60}$, $\boldsymbol n_0=(-1,0,0)^\top$, $a_0=0.02$, $U_0=\frac 1{60}$.
    \item Boundary condition: Second type condition on $\partial\mathcal D$ with $f=0$.
\end{itemize}

\subsection{Ring Collide}

\begin{itemize}
    \item Domain: $\mathcal D=[0,1]\times[0,1]\times[0,1]$.
    \item Initial velocity field:
    \begin{equation}
        \boldsymbol u(\boldsymbol x)=\boldsymbol u_\mathrm{ring}(\boldsymbol x;\boldsymbol x_1,\boldsymbol n_1,r_0,a_0,U_0)+\boldsymbol u_\mathrm{ring}(\boldsymbol x;\boldsymbol x_2,\boldsymbol n_2,r_0,a_0,U_0),
    \end{equation}
    where $\boldsymbol x_1=(\frac 5{12},0.5,0.5)^\top$, $\boldsymbol n_1=(1,0,0)^\top$, $\boldsymbol x_2=(\frac 7{12},0.5,0.5)^\top$, $\boldsymbol n_2=(-1,0,0)^\top$, $r_0=0.05$, $a_0=0.02$, $U_0=\frac 1{60}$.
    \item Boundary condition: Second type condition on $\partial\mathcal D$ with $f=0$.
\end{itemize}

\subsection{Smoking Bunny}

\begin{itemize}
    \item Domain: $\mathcal D=[0,1]\times[0,1]\times[0,1]$.
    \item Initial velocity field:
    \begin{equation}
        \boldsymbol u(\boldsymbol x)=\boldsymbol u_\mathrm{ring}(\boldsymbol x;\boldsymbol x_1,\boldsymbol n_0,r_0,a_0,U_0)+\boldsymbol u_\mathrm{ring}(\boldsymbol x;\boldsymbol x_2,\boldsymbol n_0,r_0,a_0,U_0),
    \end{equation}
    where $\boldsymbol x_1=(0.475,0.6,0.53)^\top$, $\boldsymbol x_2=(0.438,0.563,0.7152)^\top$, $\boldsymbol n_0=(0.185,0.185,-0.926)^\top$, $r_0=0.05$, $a_0=0.02$, $U_0=\frac 1{30}$.
    \item Boundary condition: Second type condition on $\partial\mathcal D$ and the surface of the Stanford Bunny with $f=0$.
\end{itemize}

\section{Hyperparameters and Normalization Strategy}

In all our examples, we use Adam optimizer with a reduce learning rate on plateau scheduler. The decaying factor of the scheduler is $0.9$, patience is $50$ for all parameters. Since we need to make sure $\boldsymbol s_i^{-1}$ is positive during the training process, we store $\tilde{\boldsymbol s}_i^{-1}=\ln(\boldsymbol s_i^{-1})$ instead of $\boldsymbol s_i$ (note that the superscription $-1$ no longer means reciprocal here).

For 2D examples, $\lambda_\mathrm{div}=1$, $\lambda_\mathrm{b1}=\lambda_\mathrm{b2}=1$, $\lambda_\mathrm{aniso}=10$, $\lambda_\mathrm{vol}=10$, $\lambda_\mathrm{pos}=0.5$, the learning rate for each parameter is as follows.
\begin{itemize}
    \item $\boldsymbol\mu_i$: $1.6\times 10^{-3}$ for initialization, $10^{-4}$ for projection, $0.01$ for reseeding.
    \item $\tilde{\boldsymbol s}_i^{-1}$: $0.05$ for initialization, $10^{-4}$ for projection, $0.05$ for reseeding.
    \item $\theta_i$: $0.05$ for initialization, $10^{-4}$ for projection, $0.05$ for reseeding.
    \item $\boldsymbol v_i$: $5\times 10^{-3}$ for initialization, $10^{-4}$ for projection, $5\times 10^{-3}$ for reseeding.
\end{itemize}

For 3D examples, $\lambda_\mathrm{div}=1$, $\lambda_\mathrm{b1}=\lambda_\mathrm{b2}=10$, $\lambda_\mathrm{aniso}=10$, $\lambda_\mathrm{vol}=10$, $\lambda_\mathrm{pos}=0$, the learning rate for each parameter is as follows.
\begin{itemize}
    \item $\boldsymbol\mu_i$: $10^{-3}$ for initialization, $3\times 10^{-4}$ for projection, $10^{-3}$ for reseeding.
    \item $\tilde{\boldsymbol s}_i^{-1}$: $10^{-3}$ for initialization, $10^{-5}$ for projection, $10^{-3}$ for reseeding.
    \item $\boldsymbol r_i$: $10^{-3}$ for initialization, $3\times 10^{-4}$ for projection, $10^{-3}$ for reseeding.
    \item $\boldsymbol v_i$: $10^{-3}$ for initialization, $10^{-5}$ for projection, $10^{-3}$ for reseeding.
\end{itemize}

We adopt a normalization strategy for the initial condition to ensure the hyperparameters are valid across different examples. Let $l_0$ be the shortest side of the fluid domain, we introduce a scaling factor $k=\frac{10}{l_0}$ in 2D and $k=\frac 1{l_0}$ in 3D. We then multiply each coordinate of the domain by $t$, along with the positions and sizes of all boundaries. The initial velocity field, $\boldsymbol u_\mathrm b$ and $f$ are substitute as follows:
\begin{align}
    &\hat{\boldsymbol u}(\boldsymbol x)=k\boldsymbol u\left(\frac{\boldsymbol x}k\right),\\
    &\hat{\boldsymbol u}_\mathrm b(\boldsymbol x)=k\hat{\boldsymbol u}_\mathrm b\left(\frac{\boldsymbol x}k\right),\text{ and}\\
    &f(\boldsymbol x)=kf\left(\frac{\boldsymbol x}k\right).
\end{align}
The gradient of the initial velocity field used in the initialization step also changes into
\begin{equation}
    \nabla\hat{\boldsymbol u}(\boldsymbol x)=\nabla\boldsymbol u\left(\frac{\boldsymbol x}k\right).
\end{equation}

\section{Special Treatment on Karman Vortex Street}

We initialize the GSR in the Karman vortex street example differently as the initial velocity field does not comply to the boundary condition. We first train the GSR with initial velocity field same as other examples, followed by a projection step with a few change to the training parameters:
\begin{itemize}
    \item Loss weights: $\lambda_\mathrm{vor}=1$, $\lambda_\mathrm{div}=10$, $\lambda_\mathrm{aniso}=10$, $\lambda_\mathrm{vol}=10$, $\lambda_\mathrm{pos}=0$.
    \item Learning rates of $\boldsymbol\mu_i$, $\tilde{\boldsymbol s}_i^{-1}$, $\theta_i$ and $\boldsymbol v_i$ are $10^{-4}$, $10^{-5}$, $1.201956\times 10^{-5}$ and $10^{-4}$, respectively.
\end{itemize}

Due to the outflow velocity of the Karman vortex street, particles are constantly carried out of the domain by the advection step, requiring supplement of particles from the inflow boundary. We fix this by initially placing sufficient particles on the left of the inflow boundary. More specifically, we expand the domain to $\mathcal D_0=[x_\mathrm{min}-Tv_0,x_\mathrm{max}]\times[y_\mathrm{min},y_\mathrm{max}]$ in the initialization step, where $T$ is the total simulation time, $v_0=0.5$ is the flow rate as specified in Section~\ref{supp:sec:karman}. We maintain a dynamic fluid domain $\mathcal D_t=[x_\mathrm{min}+(t-T)v_0,x_\mathrm{max}]\times[y_\mathrm{min},y_\mathrm{max}]$ as the domain in projection steps, where $t\in[0,T]$ is the simulation time. To maintain a constant inflow, we add another inflow boundary condition on $\{(x_\mathrm{min},y):(x_\mathrm{min},y)\in\mathcal D_t\}$.
This inflow strategy incurs a slight additional computational cost, but it is sufficient to enable the simulation to run over a long time horizon.
\section{Limitation on Vortices Pass Example}

\begin{figure}[htbp]
    \centering
    \includegraphics[trim=150 100 130 100,clip,width=1.\columnwidth]{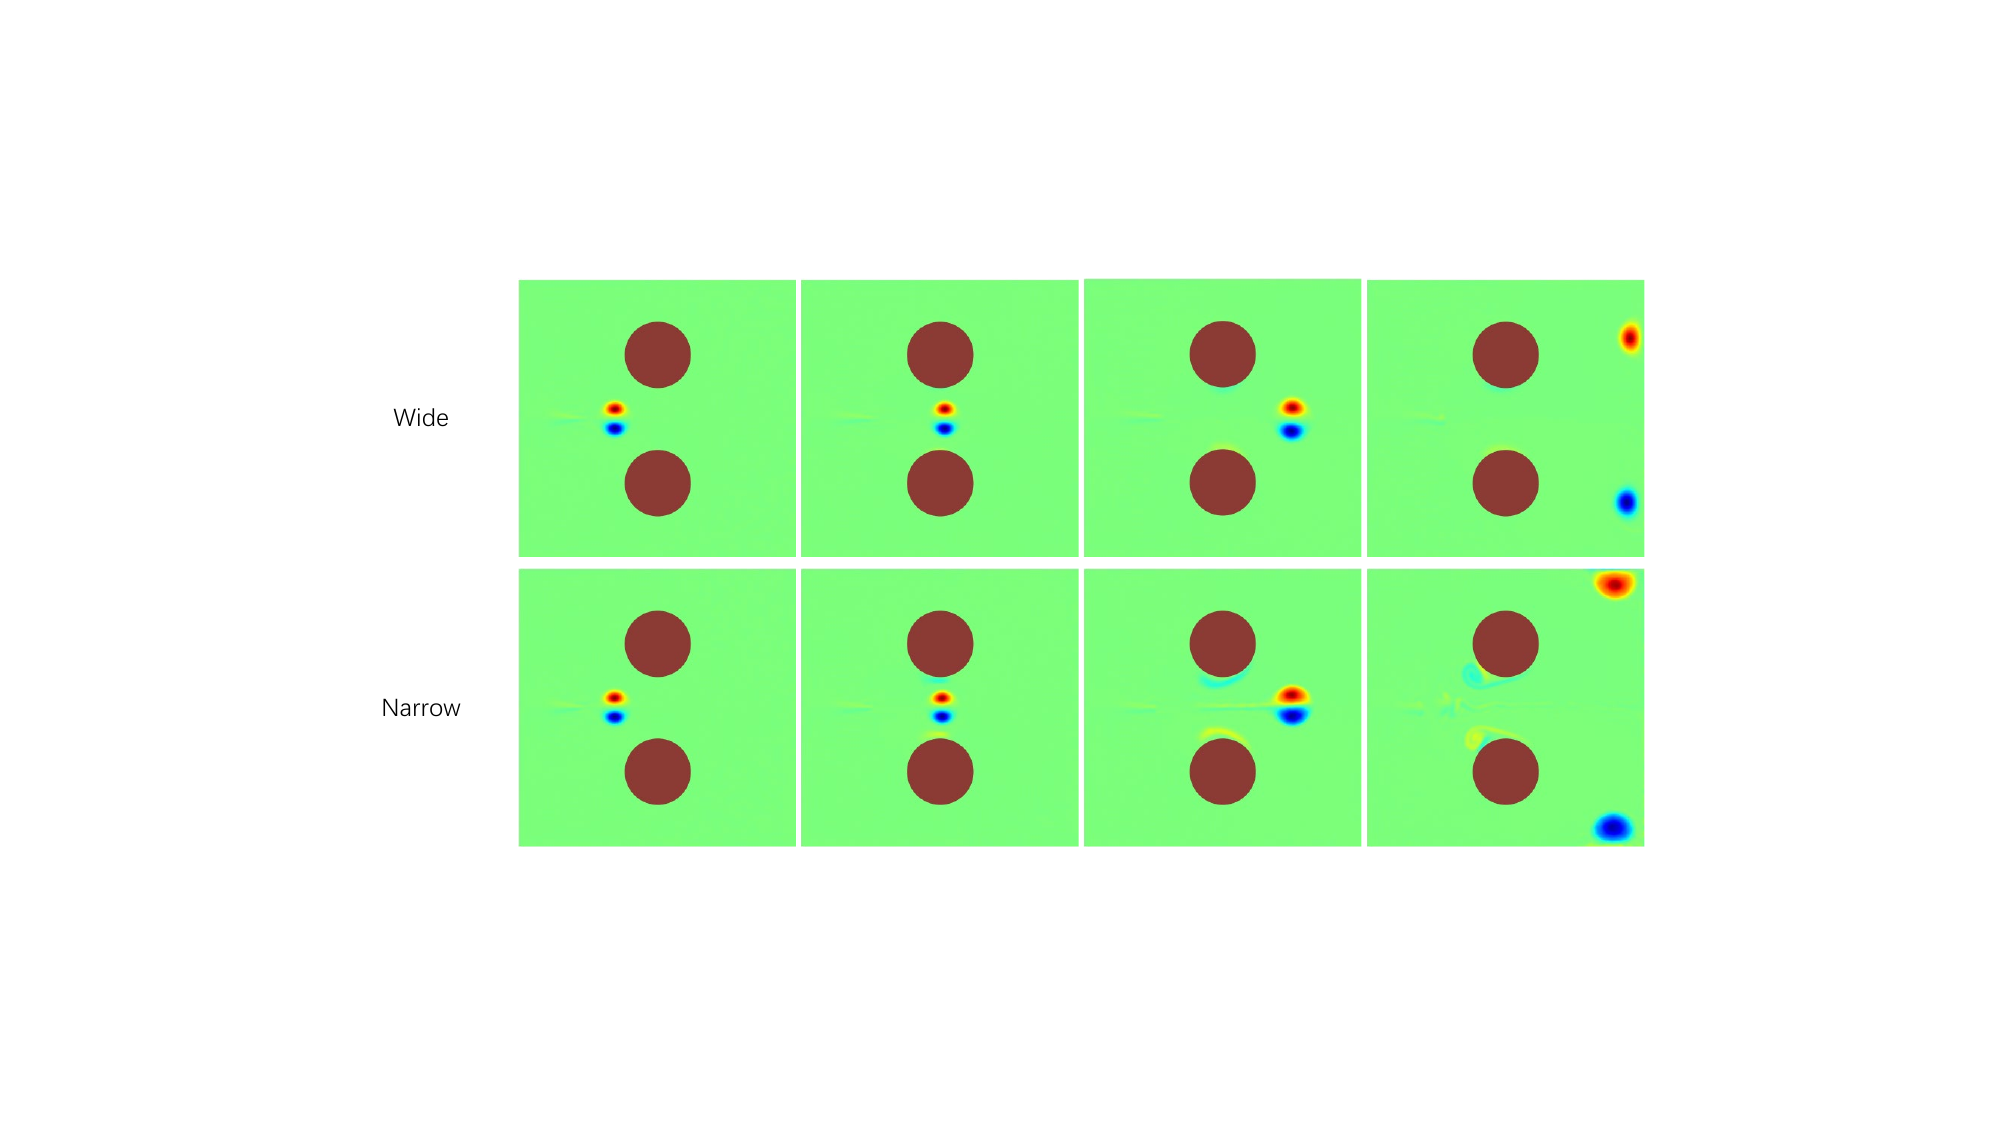}
    \caption{Simulations of the vortices pass example with wide and narrow gaps produced by our method. The wide setting is the same as the one shown in the paper, while the positions of the two spherical obstacles in the narrow setting are $(0.5,0.285)$ and $(0.5,0.715)$. The figures from left to right are showing frames 200, 336, 520 and 879, respectively.}
    \label{fig:vortices_pass-gap}
\end{figure}

\begin{figure}
    \centering
    \begin{subfigure}{.49\columnwidth}
        \centering
        \includegraphics[trim=20 0 50 0,clip,width=\textwidth]{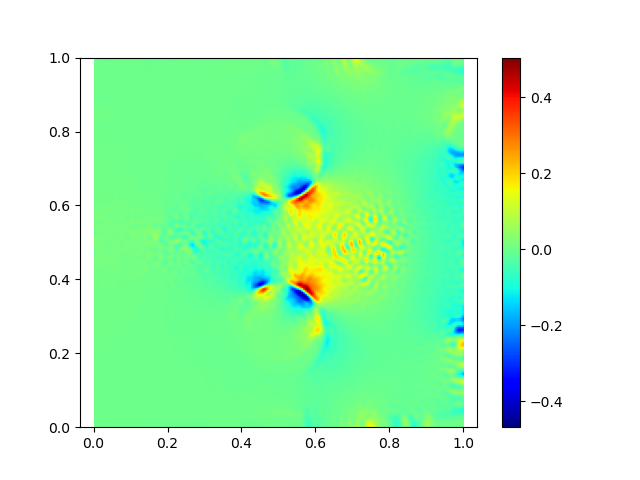}
        \caption{Wide setting}
    \end{subfigure}
    \begin{subfigure}{.49\columnwidth}
        \centering
        \includegraphics[trim=20 0 50 0,clip,width=\textwidth]{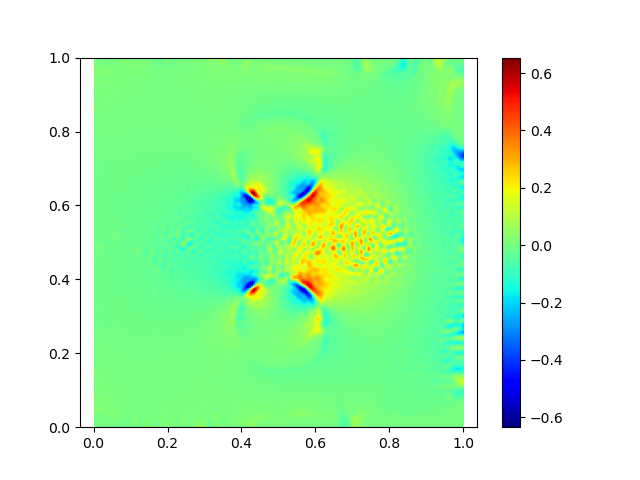}
        \caption{Narrow setting}
    \end{subfigure}
    \caption{Divergence field of the 520-th frame in the vortices pass example.}
    \label{fig:vortices_pass-div}
\end{figure}

While our method successfully allows vortex pairs to pass through gaps in the vortices pass examples, we observe a phenomenon where the vortex pair accelerates as the gap narrows (Figure~\ref{fig:vortices_pass-gap}). 
This behavior is accompanied by a greater divergence loss in the narrow gap compared to the wide gap setting(Figure~\ref{fig:vortices_pass-div}). 
It's worth noting that the divergence residual in our method is not necessarily higher than the grid-based fluid solvers, where interpolation can introduce considerable divergence at non-grid center locations.
However,  residual errors in divergence and boundary conditions can lead to discrepancies in global fluid behavior when
compared to grid-based solvers.
We hypothesize that our method may be producing behavior more akin to weakly compressible fluids in the example with a narrow gap, as the divergence loss requires more iterations due to the closer boundary condition.
In contrast, the example with a wide gap exhibits more incompressible behavior. 
While tuning hyperparameters may alleviate this issue, achieving a strictly divergence-free representation is necessary to fully resolve the problem, which we leave as a future work.
